# Supplementary material for: Chimera States in Mechanical Oscillator Networks
Source: arXiv:1301.7608 ancillary file (2013-05-27)
Supplement: Supplementary file 1 [file SupplementaryFilesV9-Compressed.pdf]

# Supporting Information

# Chimera States in Mechanical Oscillator Networks

Erik A. Martens,[1,2*†] Shashi Thutupalli,[1,3*†]
Antoine Fourrière[1], Oskar Hallatschek[1,4]

[1]Max Planck Institute for Dynamics and Self-Organization, 37077 Göttingen, Germany
[2]Institute for Aquatic Resources, Technical University of Denmark, 2800 Kgs. Lyngby, Denmark
[3]Dept. of Mechanical & Aerospace Engineering, Princeton University, Princeton, NJ 08544, USA
[4]Dept. of Physics, University of California, Berkeley, CA 94720, USA

*To whom correspondence should be addressed:
erik.martens@ds.mpg.de (E.A.M.) or shashi@princeton.edu (S.T.)
†Equal contribution

May 27, 2013

## 1 Experimental setup

### 1.1 The swing

We briefly describe the experimental setup shown in Fig. S1. Two swings are suspended by four light hollow aluminum rods of 50 cm length (outer and inner diameters are 10 mm and 9 mm, respectively). The swings are attached to the rods via low friction ball bearings to ensure smooth motion of the swings. The upper ends of the rods are attached in the same way on a large rigid support frame. The distance between the support frame and the board is set to $L = 22$ cm. The motion of the two swings (A and B) is constrained so that it (to high precision) can only occur in the $(x, y)$-plane along the arc lengths $S_A = L\Psi$ and $S_B = L\Phi$, respectively. Each swing is made of a 500 mm x 600 mm x 1 mm perforated aluminum plate. To make the plates stiff and flat, they are bent at the edges and aluminum tubes of square cross-section are placed underneath the board for further support. The total mass of each plate is $m_s = 915$ g $\pm 4$ g.

Each swing is loaded with $N = 15$ metronomes of mass $m_m = m + m_{\text{box}} = 93$ g, where $m = 28$ g is the mass of the entire metronome pendulum (composed of a larger rigid part, $m_p = 23$ g and a smaller adjustable bob, $m_{\text{bob}} = 5$ g to set the frequency); $m_{\text{box}} = 65$ g is the mass of the metronome's box (see Fig. S3). Thus, the total mass of swing and metronomes amounts to $M = m_s + N \times m_m \approx 2.3$ kg.

The adjacent swing rods (two pairs at the front and back side of the swing) are connected with two precision metallic springs (the back pair of rods is shown in Fig. S2A). The pivots of two adjacent rods are set to a distance of $L_p = 20$ cm. The springs used in our study (Febrotec GmbH, Germany) have the following characteristics: an outside diameter of 6.14 mm, wire diameter of 0.46 mm, unloaded length of 38.1 mm, preload force of 0.41 N and force at a length of 152.2 mm: 4.37 N. For a single spring, we

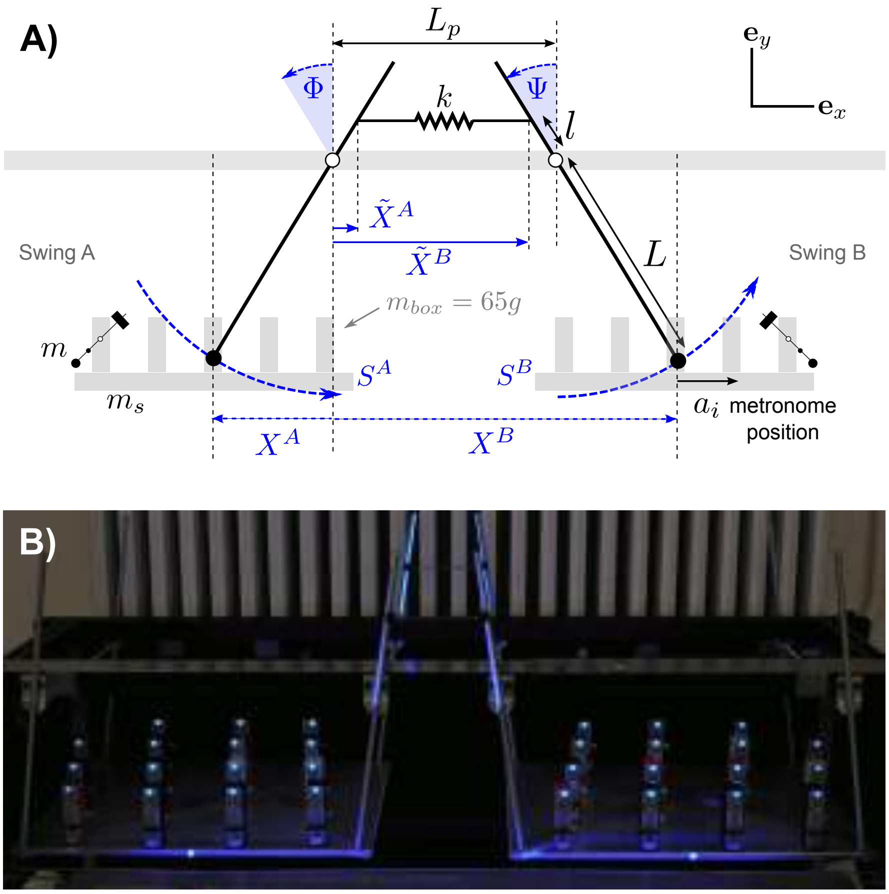


Fig. S 1: System with two swings coupled with two identical springs. Each swing carries $N = 15$ metronomes. **A:** Schematics of experimental setup. **B:** Each swing and the *top* of each pendulum are marked with fluorescent dots, which are highlighted using UV light. Note that the center mass motion occurs in opposite direction of these dots since the center mass of the metronome pendulum lies below its pivot (see Fig. S3).

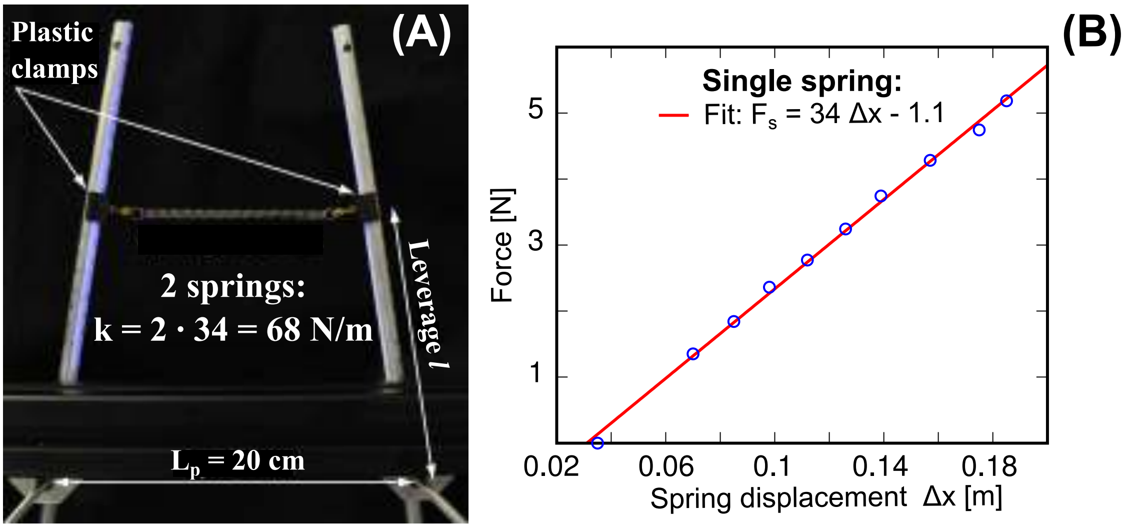


Fig. S 2: **A:** Two springs mediate the coupling between the two adjacent rod pairs at the front and back sides of the swings (back side shwon). The springs are firmly connected to the rods with plastic clamps. **B:** The spring constant of a single spring in or setup has been measured with a value of 34 $N.m^{-1}$, thus the resulting total spring rate is $k = 68\ N.m^{-1}$ with two springs attached.

measured a rate of 34 $\mathrm{N.m}^{-1}$ (see Figure S2.B), thus the total spring rate yielded by the two springs used in our setup is $k = 68\ \mathrm{N.m}^{-1}$. Both springs are attached to plastic clamps at both ends (see Figure S2.A); the clamps are firmly attached to the rods at distance $l$ above the pivot point. The clamps can be slided up and down while still being firmly fixed to the rods during an experiment. Thereby we change the spring lever $l$ and the associated torque, i.e. we effectively tune the spring coupling strength.

**Swing equilibrium angle.** The swing positions $\Phi, \Psi$ can be parametrized with small amplitude variations $\Phi', \Psi'$ around their equilibrium angles $\Phi^*, \Psi^*$, i.e.,

$$\Phi'(t) = \Phi(t) - \Phi^*, \tag{1}$$

$$\Psi'(t) = \Psi(t) - \Psi^*, \tag{2}$$

which are $\sim 1^\circ \ldots 2^\circ$. Typical equilibrium angles with varying spring leverage $l$ are summarized in Table 1; their magnitude is small which allows us to make the small angle approximations further below. The equilibrium torque balance defines an equilibrium spring force $\tilde{F}_s^*$:

$$l\ \tilde{F}_s^* = -L\ Mg\ \sin\Phi^*. \tag{3}$$

Note that $\Psi^* = -\Phi^* < 0$ due to the symmetry of the setup.

**Swing friction.** To experimentally estimate the friction coefficient in the swing, we observe the equation of motion for one swing:

$$\partial_t^2 \Phi = -\frac{g}{L}\ \sin\Phi - \frac{\nu_s}{M}\ \partial_t \Phi\,. \tag{4}$$

The eigenfrequency of the swing is $\Omega = \sqrt{g/L} \approx 6.67\ \mathrm{rad.s}^{-1}$. For small angles $\sin\Phi \approx \Phi$, we obtain the solution

$$L\ \Phi(t) = L\ \Phi_0\ e^{-\nu_s\, t/(2\,M)}\ \cos\left[\sqrt{\Omega^2 - (\nu_s/4M)^2}\ t\right]. \tag{5}$$

| $l$ [cm] | $\Phi^*$ [deg] |
|---|---|
| 7 | 5.3 |
| 10 | 6.9 |
| 11 | 7.3 |
| 14 | 8.2 |
| 20 | 9.2 |
| 23 | 9.0 |

Table 1: Typical equilibrium angles with varying spring lever $l$. Measurements for the equilibrium angle are performed with $L_p = 0.2$ m, $L = 0.22$ m, $M = 2.3$ kg and $k = 68$ N/m.

We infer the friction coefficient $\nu_s$ by measuring the evolution of the amplitude of the swing $L\ \Phi(t)$, initially removed from its equilibrium position by an angle $\Phi(0) = \Phi_0$ and released without any celerity, $\partial_t \Phi(0) = 0$. By observing the decaying amplitude $L\Phi(t)$ over a few minutes and comparing the data with (5), we find that typically $\bar{\nu}_s \sim 0.1$ kg/s.

## 1.2 The metronome

The working principle behind the metronome mechanism is identical to Huygens' pendulum clocks (Ref. [41]), except that the escapement in the metronome is driven by a spring rather than a mass pulled by gravity. While friction inherent to the mechanical elements attenuates large amplitude oscillations towards the nominal metronome oscillation amplitude, small pendulum oscillations are amplified by the spring energy feeding the pendulum via the escapement mechanism. Together, this gives the metronome the characteristics of a self-sustained oscillator (Ref. [42]).

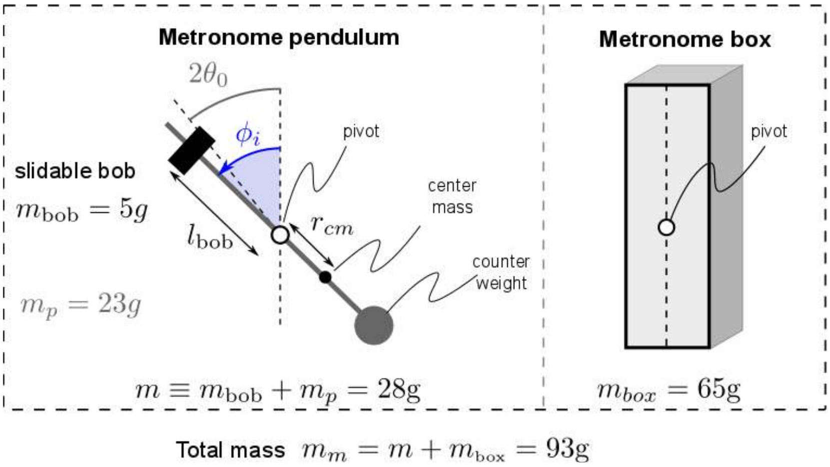


Fig. S 3: The metronome has two components: (left) the metronome pendulum of mass $m$ constitutes the dynamically active element of the metronome system, and (right) the metronome box of mass $m_{box}$ which is fixed with respect to the swing system. The state of the metronome pendulum is described by its displacement angle $\phi_i$ and its angular velocity $\partial_t \phi_i$. $\theta_0$ is half the standard displacement angle of the pendulum (single uncoupled pendulum). The pendulum is composed of a counterweight (gray disk) and rod (gray) of mass $m_p$; the frequency of the pendulum is adjusted by sliding the bob mass $m_{\text{bob}}$ (black rectangle) above the pivot (empty circle) up and down, resulting in an alteration of the pendulum's center mass position $r_{cm}$ which always lies below the pivot.

In our experiment, we employ Wittner's Super-mini Taktell metronomes used in previous studies (Ref. [42]), covering a frequency range of 40 (Largo) to 208 (Prestissimo) beats per minute (bpm) with a standard deviation of relative frequencies of ∼1%. Each metronome has physical dimensions of 30 mm x 37 mm x 104 mm and mass $m_m = 93$ g. When fully wound up, each metronome ticks for a duration of $\sim 20$ minutes (depending on the adjusted frequency $f$), corresponding to $\sim 1500$ oscillation cycles.

During operation, each metronome is firmly attached on the swing plate with double-sided Scotch tape; their standard position is marked with a pen on the swing boards such that we maintain the same arrangement of metronomes on the plate for each experiment. The total mass of the swing is $M = m_s + N \times m_m = 2.3$kg. To record the angle displacement of each metronome, $\phi_i$ and $\psi_i$, from the swing $A$ and $B$ respectively, small round stickers of diameter $\sim 10$ mm are attached at the upper part of the rod. The stickers are UV fluorescent which allows digital tracking of the metronome motion. We checked that their addition (negligible mass) does not change the metronome characteristics relevant to the observations made here.

The metronome may be conceptually split into two parts: i) the rigid, non-moving box of mass $m_{\text{box}}$, containing the spring and escapement mechanism driving the pendulum; ii) the oscillating pendulum of mass $m_p$. It is composed of a rod with a weight attached on the lower end (the counter-weight); on the top end, there is a second weight (bob) that can be moved up and down (see Figure S3).

**Frequency.** The only control parameter of the metronome is its beating frequency: it is adjusted by sliding the bob up and down, thereby altering the first (center mass $r_{\text{cm}}$) and second moment of the metronome pendulum, $I$.

The (quasi-)linear eigenfrequency $\omega$ of the metronome (33) is not exactly equal to the nominal frequency $f$ of the nonlinear oscillator. The relationship between the two frequencies can be estimated by considering higher order expansions of the sine-term and the van-der-Pol term in the governing equations (28). A first order estimate of the nominal frequency is given by (Refs. [42, 43]):

$$\omega_n = \left[1 - \left(\frac{\theta_0}{2}\right)^2\right] \omega, \tag{6}$$

The angular frequencies $\omega$ and $\omega_n$ are measured in rad.s$^{-1}$ rather than in beats per minute (bpm). The conversion between the two units is given via $\omega = f \cdot \pi/60$ (2 beats correspond to one oscillation period). $\theta_0 \approx 19^\circ$ is half the standard displacement angle of the pendulum (see model below).

**Center mass and second moment of inertia.** The first and second moments of inertia enter as parameters in the model that we develop further below. We need to determine the relationship between these moments and the metronome frequency $f$ which we use as an experimental control parameter. Determining the two moments by disassembling the pendulum into separate parts (bob, pendulum rod, counterweight, axle, axle-to-rod connector) and measuring their mass and relative positions results in a tedious estimation exercise, and is prone to undue error[1].

We therefore resort to a simple parameter fit, based on first principles and few empirical measurements. We measure all distances relative to the pivot, so that positions on the upper part of the pendulum rod are positive. Let us denote $l_{\text{bob}}$ the distance of the bob to the pivot (axle) of the metronome (the bob's center mass is located about 5 mm below its upper edge). The center mass of the pendulum is then located at $r'_{\text{cm}} = (m_0 l_0 + m_{\text{bob}} l_{\text{bob}})/m = r_0 + m_{\text{bob}}/m \cdot l_{\text{bob}}$ and the second moment of inertia is $I = m_0\, l_0^2 + m_{\text{bob}} l_{\text{bob}}^2 = I_0 + m_{\text{bob}} l_{\text{bob}}^2$. The mass of the bob is $m_{\text{bob}} = 5$ g and the mass of the entire pendulum is $m = 28$ g. To determine $r_0$, we detach the pendulum from its box, and set the bob to the maximum position at $l_{\text{bob}} \approx 26$ mm at frequency f $= 208$ bpm. We then balance the pendulum on the

[1] To achieve accurate nominal frequencies, the bobs are manually calibrated, i.e. the manufacturer filed each pendulum bob individually to fit; a reflection of the high sensitivity on small mass and geometric variations.

edge of a razor blade and find that $r_{\rm cm} \approx -7.5$ mm, corresponding to $r_0 = -12.1$ mm. We thus have the (by definition) *positive* center mass distance

$$r_{\rm cm} \approx \Big| -0.0121 \text{ m} + 0.178 \cdot l_{\rm bob} \text{ [m]} \Big| > 0. \quad (7)$$

The second moment of inertia is related to the quasilinear eigenfrequency $\omega$ via Eq. (33), $I = mg\, r_{\rm cm}\, \omega^{-2}$, which we evaluate for $f = 208$ bpm by using the above approximation for $r_{\rm cm}$ and (10) below,

$$I_0 = I|_{f=208} - m_{\rm bob}\, l_{\rm bob}^2 = 1.29 \times 10^{-5} \,\text{kg}\,\text{m}^2. \quad (8)$$

We then have

$$I = 1.29 \times 10^{-5} \text{ kg m}^2 + 5 \times 10^{-3} \text{ kg} \cdot l_{\rm bob}^2 [m^2]. \quad (9)$$

Finally, by simply reading off values for $l_{\rm bob}$ for given nominal frequencies $f$, we find the following linear fit

$$l_{\rm bob} \approx 7.3 \times 10^{-2} \text{ m} - 2.2 \times 10^{-4} \text{ m/bpm} \times f \text{ [bpm]}, \quad (10)$$

which turns out to be approximately linear for the frequency range considered. Combination of Eqs. (7-10) yields the required relationship for $I = I(f)$ and $r_{\rm cm} = r_{\rm cm}(f)$.

# 2 Experimental methods

## 2.1 Experimental protocol

An experiment is started with a careful symmetry check of the system: the two uncoupled boards are displaced from their equilibrium position (in the uncoupled case, at equilibrium, the rods are vertical: $\Phi^* = \Psi^* = 0$) and released at the same time. By observing the decrease of amplitude $L\Phi(t)$ and $L\Psi(t)$, we check that the initial friction $\nu_s$ is the same on both swings. All the metronomes are then wound up and their nominal frequency $\omega_n$ is adjusted to the same value and double checked. Then the metronomes are firmly and precisely placed on each board. We then connect the two swings with the spring which is firmly set at a distance $l$ above the pivot points. The metronomes are put in motion. The initial conditions are prepared to be compliant to one of two states: (i) DS (equivalently, SD) corresponding to desynchrony and synchrony on the left or right swings, respectively ; or ( ii) both populations are started in desynchrony (DD). The desynchrony of the population on one swing is ensured by blocking the motion of the swing physically; meanwhile, the other population on the other swing achieves full synchrony via its free swing motion. The start of an experiment is then marked by the time point when this swing is released. The motion of the metronomes and the swings is recorded by video recording under UV illumination using a Nikon D90 camera mounted with an $18-55$ mm lens (DX format). After the experiment, we repeat the protocol for the very same parameters and we invert the roles of the swings (i.e. a DS experiment is followed by an SD experiment), so that the left-right symmetry is checked thoroughly.

## 2.2 Data Analysis

The videos from the experiment are further processed to extract quantitative information by image processing using MATLAB. The metronome pendulums and the swings are marked by UV fluorescent spots (see Fig. S1B). These bright spots show up as circular white regions in the images, which are then tracked by their centroids to obtain the positions $x(t)$ and $y(t)$ of the metronome pendula as a function of time. The phases $\theta_k^{(1)}(t)$ and $\theta_k^{(2)}(t)$ of the metronomes and $\Theta^{(1)}(t)$ and $\Theta^{(2)}(t)$ of the swing oscillations on population 1 and 2, respectively, are obtained from the time tracks of those positions using

the Hilbert transform in MATLAB (this technique works well as the signal is sufficiently narrow-banded, see Refs. [44, 45]),

$$H\left[x_k^{(p)}(t) - X^{(p)}(t) - \left\langle (x_k^{(p)}(t) - X^{(p)}(t) \right\rangle_t \right]$$
$$= \pi^{-1} \int_{-\infty}^{\infty} \left[x_k^{(p)}(t') - X^{(p)}(t') - \left\langle x_k^{(p)}(t') - X^{(p)}(t') \right\rangle_t \right] / (t - t')\, dt' \qquad (11)$$

where $x_k^{(p)}(t)$ is the position of the $k^{th}$ metronome bob on swing $p = 1, 2$ and $X^{(p)}(t)$ is the position of the swing on which the metronome is attached, and $\left\langle x_k^{(p)}(t) - X^{(p)}(t) \right\rangle_t$ is its temporal mean that we subtract from the signal to center the data around the origin. The Hilbert transform allows us to reconstruct the analytic representation of the signal $x(t)$, i.e., $x_a(t) = x(t) + iH(x)(t)$; for a narrow-banded signal, we then have $x_a(t) = A(t)e^{i[\omega t + \theta(t)]}$. The phases $\theta_k(t)$ are used to calculate time-averaged frequencies and to quantify the synchronization using the Kuramoto order parameters for populations $p = 1, 2$,

$$Z_p(t) \equiv \frac{1}{N} \sum_{k=1}^{N} \exp\{i[\theta_k^{(p)}(t) - \bar{\theta}_{\text{syn}}^{(p)}(t)]\}, \qquad (12)$$

where $\bar{\theta}_{\text{syn}}(t)$ is the average phase of the synchronous population at time $t$. Further, the phases are used to obtain the average frequencies over a time window $T$, i.e. $\omega_k \approx [\phi_k(T) - \phi_k(0)]/T$. These frequencies may be compared to the average frequency of the synchronous population, $\bar{\omega}_{\text{syn}} \equiv N^{-1} \sum_{k=1}^{N} \omega_k$.

# 3 Further experimental results

In addition to the chimera behavior, we also find other collective modes. For instance, a phase-clustered state is shown in Fig. S4. The relative frequencies of the synchronized and desynchronized populations reveal the presence of distinct frequency clusters in the desynchronized population. A snapshot of the metronome phase for the synchronized population, S and the desynchronized population further reveals the existence of 4 phase clusters $\mathrm{C}_1, \mathrm{C}_2, \mathrm{C}_3$ and $C_4$ within the desynchronized population. To analyze these clusters in more detail, we calculate the order parameter $Z(t)$, for each of the clusters individually. While cluster $\mathrm{C}_1$ is locked in anti-phase with S, clusters $\mathrm{C}_2, \mathrm{C}_3$ and $\mathrm{C}_4$ are not phase locked with respect to S. However, the clusters $\mathrm{C}_3$ and $\mathrm{C}_4$ are locked roughly in anti-phase with each other, while still drifting with respect to S. It is remarkable to note that these various complex dynamics within the desynchronized population all together give rise to a time varying order parameter which, after an initial transient, appears highly periodic.

All experimental states have been examined in a manner as outlined above; in particular, for the chimera states we have ensured that phase locking between any of the individual oscillators within the asynchronous population is absent.

# 4 Model

The dynamics of the two swings is described by the angles $\Phi(t)$ and $\Psi(t)$ and their corresponding angular velocities (see Figs. S1 and S5), which describe the motion along arc coordinates $S_A = L\Phi$ and $S_B = L\Psi$. The motion of the metronome pendula is described by their displacement angles $\phi_i(t)$ on swing $A$ and $\psi_i(t)$ on swing $B$, respectively. As explained above, to set up the governing equations, we conceptually divide the system into two sub-systems: i) the system of the two coupled swings ii) the system of the $N$ metronomes populating each swing. For all angles we use mathematically positive orientation, see Figures S1 and S3.

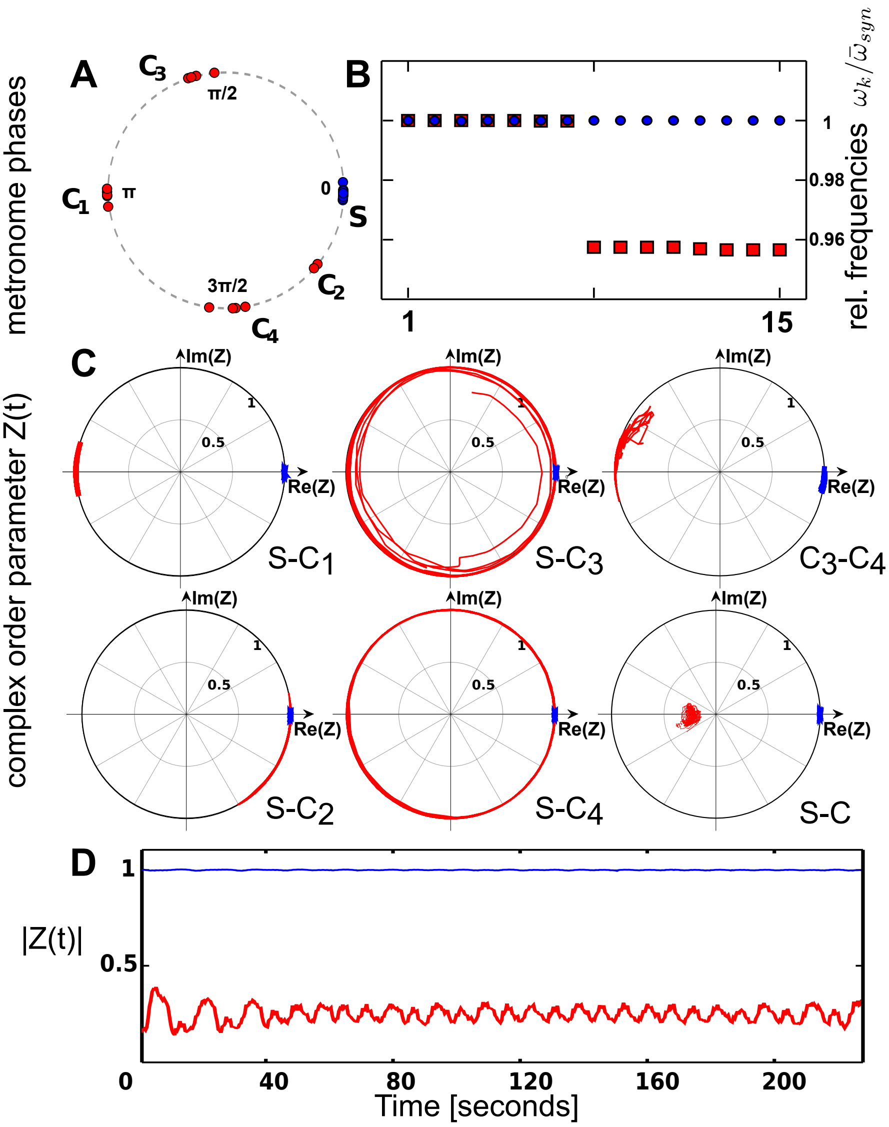


Fig. S 4: Analysis of a (partially) phase-clustered state obtained for inter-population coupling of $\kappa = 29.56$ and nominal metronome frequency f = 184 beats per minute (bpm). **A:** Phases of individual metronomes (red: asynchronous population; blue: synchronous population(S)). Phases belonging to different clusters are shaded in gray and labeled $C_i$. **B:** Frequencies averaged over the last 50% of the observation time, $\bar{\omega} = \langle \omega \rangle_t$, relative to the average frequency $\bar{\omega}_s$ of the synchronized population; red and blue populations are superponed. **C:** Complex order parameter of the subpopulations $C_i$ relative to order parameter of the synchronized population (i.e., the angular component is subtracted - thus a view in the co-rotating frame is shown.) **D:** Time evolution of the magnitude of the order parameters of the synchronous and asynchronous population.

## Swing system

We derive equations of motion for the two swings by considering the external forces acting on the center mass system of swing $A$ (and $B$, respectively),

$$M\partial_t^2 \begin{pmatrix} X_{\rm cm}^A \\ Y_{\rm cm}^A \end{pmatrix} = \mathbf{F}_{\rm ext}^A \tag{13}$$

The center mass system is comprised of the swing board of mass $m_s$ and the metronomes of mass $m_m$, i.e. $M = m_s + N \cdot m_m = m_s + N(m_{\rm box} + m_p)$. The masses of the suspension rods are negligible in comparison to the mass of the swings and the metronomes $M$. The external force acting on the center

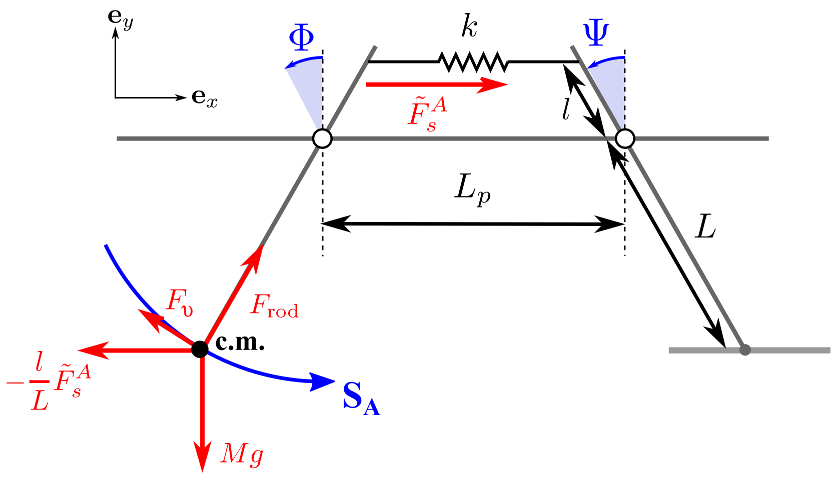


Fig. S 5: Free body diagram of the swing's center mass system. The swing center mass system includes the metronome pendula and does not exactly coincide with the center mass of the board.

mass system is composed of the sum $\mathbf{F}_{\rm ext}^A = \mathbf{F}_g^A + \mathbf{F}_s^A + \mathbf{F}_\nu^A + \mathbf{F}_{\rm rod}^A$, i.e. the sum of the following forces (see Figure 5):

**i) Gravity:**

$$\mathbf{F}_g^A = -\, M\, g\, \hat{\mathbf{e}}_y \tag{14}$$

**ii) Spring force:**

$$\mathbf{F}_s^A \;=\; -\frac{l}{L}\tilde{\mathbf{F}}_s^A = -\frac{l}{L}[\tilde{F}_s^* + k\, l(\Phi' - \Psi')]\hat{\mathbf{e}}_x \tag{15}$$

where $\Phi', \Psi'$ are the displacement angles measured from the equilibrium and $\tilde{F}_s^*$ is the equilibrium spring force defined in Eq. 3.

**iii) Friction:** The swing friction force is given by

$$\mathbf{F}_\nu^A \;=\; -\,\nu_s\, \partial_t S_A\, \hat{\mathbf{e}}_s = -\,\nu_s\, L\partial_t\Phi\, \hat{\mathbf{e}}_s\,, \tag{16}$$

where we introduce the unit vector $\hat{\mathbf{e}}_s = (\cos\Phi, \sin\Phi)$.

**iv) Rod force:** The force exerted by the pendulum rods that constrain the motion is

$$\mathbf{F}_{\rm rod} \;=\; [-(\mathbf{F}_g^A + \mathbf{F}_s^A + \mathbf{F}_\nu^A)\cdot \hat{\mathbf{e}}_r]\,\hat{\mathbf{e}}_r \tag{17}$$

where we introduce the unit vector $\hat{\mathbf{e}}_r = (\sin\Phi, -\cos\Phi)$ perpendicular to $\hat{\mathbf{e}}_s$ (this force cancels later).

**Center mass system.** The x-component of the center mass location of swing $A$ is given by

$$MX_{\rm cm}^A \;=\; (m_s + Nm_{box})X^A + m\sum_{j=1}^{N}(X^A + x_j^A) = MX^A + m\sum_{j=1}^{N} x_j^A,$$

where $X^A \equiv L\sin\Phi$ and $X^B \equiv L_p + L\sin\Psi$ are the positions of swing $A$ and $B$, respectively; here we have merged the masses of the rigid parts of the metronome mass (i.e., the box) with that of the swing, $m_s$. The center mass of each pendulum $k$ is relative to swing $A$ located at

$$x_j^A \;=\; a_k \;+\; r_{\rm cm}\;\sin\phi_j\,, \tag{18}$$

where $a_k$ are the positions of metronome $k$ on the swing board; $r_{\rm cm}$ is the distance of the center mass of the pendulum relative to its pivot, and $\phi_k$ is the angle of metronome $k$ on swing $A$ with the vertical axis (see Fig. S3). This allows us to express the inertia of the swing's center mass system in terms of the swing coordinate and the metronome coordinates $x_k$. We thus have

$$M\partial_t^2 X_{\rm cm}^A \;=\; M\partial_t^2 X^A + m\sum_{j=1}^{N}\partial_t^2 x_j^A\;. \tag{19}$$

Since all metronomes are firmly attached to the swing, i.e. $\partial_t a_k = 0$, we obtain

$$M\partial_t^2 X_{\rm cm}^A \;=\; M\partial_t^2 X^A + mr_{\rm cm}\sum_{j=1}^{N}\partial_t^2\sin\phi_j, \tag{20}$$

$$M\partial_t^2 Y_{\rm cm}^A \;=\; M\partial_t^2 Y^A + mr_{\rm cm}\sum_{j=1}^{N}\partial_t^2\cos\phi_j, \tag{21}$$

where the latter is the analogous expression for the center mass position in y-direction.

Projection of the force balance (13) onto $\hat{\mathbf{e}}_s$ yields

$$ML(\cos\Phi\,\partial_t^2\sin\Phi + \sin\Phi\,\partial_t^2\cos\Phi) + mr_{\rm cm}\sum_{j=1}^{N}(\cos\Phi\,\partial_{tt}\;\sin\phi_j + \sin\Phi\,\partial_{tt}\;\cos\phi_j)$$
$$= -Mg\sin\Phi - \frac{l}{L}[\tilde{F}_s^* + kl(\Phi' - \Psi')]\cos\Phi - \;\nu_s\,L\partial_t\Phi. \tag{22}$$

**Small angle approximation.** The displacements $\Phi, \Psi$ of the two swings are small, and in particular, the swings make small amplitude oscillations ($\sim 1^\circ$ to $2^\circ$) around their equilibrium positions $\Phi^*$ and $\Psi^*$ in Eq. (1)), viz.

$$\Phi(t) \;=\; \Phi^* + \Phi'(t)\,,$$
$$\Psi(t) \;=\; \Psi^* + \Psi'(t)\,.$$

In our experiments, the equilibrium angles lie in a range from 5° to 10°, see Table 1. In the following, we shall therefore use the small angle approximations $\sin\Phi = \Phi + \mathcal{O}(\Phi^3)$ and $\cos\Phi = 1 + \mathcal{O}(\Phi^2)$. The approximated dynamics is then given by

$$ML\partial_t^2\Phi + mr_{\rm cm}\sum_{j=1}^{N}(\partial_{tt}\,\sin\phi_j + \Phi\,\partial_{tt}\,\cos\phi_j)$$
$$= -Mg\Phi - \frac{l}{L}[\tilde{F}_s^* + kl(\Phi' - \Psi')] - \;\nu_s\; L\partial_t\Phi. \tag{23}$$

Further, we simplify the equation by observing that $|\sum_{j=1}^{N}\partial_{tt}\,\sin\phi_j| \gg |\Phi\cdot\sum_{j=1}^{N}\partial_{tt}\,\cos\phi_j| \sim |\Phi|$, and by parameterizing the swing angles in terms of their equilibrium angles, Eqs. (1):

$$ML\partial_t^2\Phi' + mr_{\rm cm}\sum_{j=1}^{N}\partial_{tt}\,\sin\phi_j$$
$$= -Mg(\Phi^* + \Phi') - \frac{l}{L}[\tilde{F}_s^* + kl(\Phi' - \Psi')] - \;\nu_s\; L\partial_t\Phi'. \tag{24}$$

Cancellation of the swing equilibrium force $\tilde{F}_s^*$ in Eq. (3) and noting that $\Psi^* = -\Phi^* > 0$ yields the governing equations for swings A and B:

$$\partial_t^2\Phi' \;=\; -\frac{g}{L}\Phi' + \frac{k}{M}\frac{l^2}{L^2}(\Psi' - \Phi') - \frac{\nu_s}{M}\partial_t\Phi' - \frac{m\,r_{\rm cm}}{M\,L}\sum_{j=1}^{N}\partial_t^2\sin\phi_j, \tag{25}$$

$$\partial_t^2\Psi' \;=\; -\frac{g}{L}\Psi' + \frac{k}{M}\frac{l^2}{L^2}(\Phi' - \Psi') - \frac{\nu_s}{M}\partial_t\Psi' - \frac{m\,r_{\rm cm}}{M\,L}\sum_{j=1}^{N}\partial_t^2\sin\psi_j. \tag{26}$$

## Metronome system

To close Eqs. (25-26), we need to describe the motion of the angles of the pendula on the swings A and B. The pendulum angles with the vertical are denoted by $\phi_i$ and $\psi_i$ for populations on swing $A$ and $B$, respectively (see Fig. S3). We have

$$0 \;=\; I\,\partial_t^2\,\phi_i + mg\,r_{\rm cm}\sin\phi_i + \nu_m\,\partial_t\,\phi_i\left[\left(\frac{\phi_i}{\theta_0}\right)^2 - 1\right] + mr_{\rm cm}\cos\phi_i\,\partial_t^2 X^A\,, \tag{27}$$

and the analogous equations for $\psi_i$. The first term is the rotational inertia with the second moment $I = \int\rho(r)r^2dV$, and the second term is due to gravity with the first moment $r_{cm}$ of the metronome pendulum. The two moments $r_{cm}$ and $I$ are parametrized in terms of the metronome frequency $f$, see Eqs. (7,9,10) further above. The third term is a van der Pol term which is commonly used in literature to model the escapement mechanism (see e.g. Refs. [41, 46, 47] or Pantaleone [42] who uses the same make of metronomes as we do here). The van der Pol term is parameterized with two parameters $\nu_m$ and $\theta_0$. $2\theta_0$ is the standard displacement angle of an uncoupled, non-accelerated metronome pendulum ($2\theta_0 = 37° - 38°$ ) mounted on a horizontal surface. The resulting dissipation is amplitude-dependent and switches sign depending on the magnitude of the metronome's displacement angle: when the pendulum displacement $\phi_i > \theta_0$, energy is dissipated whereas in the opposite case, the motion of the pendulum is amplified (escapement mechanism transfers spring energy to the pendulum); in effect, the oscillation assumes a limit cycle oscillation. Even though the term is *ad-hoc*, it is (qualitatively) generic in the sense that it may be considered a symmetric expansion of a dissipation term of the type $\partial_t\phi\cdot f(\phi)$ to second order in $\phi$, where $f(\phi)$ must be symmetric [note though that the tilting of a metronome – so it is not

standing vertically – results in asymmetric ticking (long-short-long-...)]. The van-der-Pol-term may also be thought of as a time-average proxy of the discrete process performed by the escapement.

Finally, the last term comes from the inertia exerted from the center mass swing motion. The torque is computed via the projection of the swing motion in x-direction into the arc coordinates, i.e. $m\, r_{\text{cm}} \cos\phi_i\, \partial_t^2 X$. The center mass of swing $A$ is

$$M\, X^A \;=\; M\, L \sin\Phi = ML(\Phi^* + \Phi') + \mathcal{O}(\Phi^3).$$

Thus, neglecting higher order terms, we have $\partial_t^2 X^A \approx L\, \partial_t^2 \Phi'$ and we get

$$\partial_t^2 \phi_i \;=\; -\frac{m\, g\, r_{\text{cm}}}{I} \sin\phi_i - \frac{\nu_m}{I}\, \partial_t \phi_i \left[ \left( \frac{\phi_i}{\theta_0} \right)^2 - 1 \right] - \frac{m\, r_{\text{cm}}}{I} L \cos\phi_i \partial_t^2 \Phi' \tag{28}$$

plus the corresponding equations for the metronome angles $\psi_i$ on swing B.

## Summary

The resulting governing equations may be further cast into a simpler form amenable to physical interpretation of parameters by introducing the rescaled time $\tau = \omega t$:

$$\partial_\tau^2 \Phi' \;=\; -\left(\frac{\Omega}{\omega}\right)^2 \Phi' + \frac{\kappa}{\omega^2}(\Psi' - \Phi') - \mu_s \partial_\tau \Phi' - \frac{x_0}{L} \sum_{j=1}^{N} \partial_\tau^2 \sin\phi_j \tag{29}$$

$$\partial_\tau^2 \Psi' \;=\; -\left(\frac{\Omega}{\omega}\right)^2 \Psi' + \frac{\kappa}{\omega^2}(\Phi' - \Psi') - \mu_s \partial_\tau \Psi' - \frac{x_0}{L} \sum_{j=1}^{N} \partial_\tau^2 \sin\psi_j \tag{30}$$

$$\partial_\tau^2 \phi_i \;=\; -\sin\phi_i - \mu_m\, \partial_\tau \phi_i \left[ \left( \frac{\phi_i}{\theta_0} \right)^2 - 1 \right] - \frac{\omega^2 L}{g} \cos\phi_i\, \partial_\tau^2 \Phi', \tag{31}$$

$$\partial_\tau^2 \psi_i \;=\; -\sin\psi_i - \mu_m\, \partial_\tau \psi_i \left[ \left( \frac{\psi_i}{\theta_0} \right)^2 - 1 \right] - \frac{\omega^2 L}{g} \cos\psi_i\, \partial_\tau^2 \Psi', \tag{32}$$

where we have dropped the primed notation in the main text. The rescaled parameters are

$$\begin{aligned} \mu_m &\equiv \frac{\nu_m}{I\omega}, \\ \mu_s &\equiv \frac{\nu_s}{M\omega}, \\ \omega^2 &\equiv \frac{mg\, r_{\text{cm}}}{I}, \\ \Omega^2 &\equiv \frac{g}{L}, \\ \kappa &\equiv \frac{k}{M} \frac{l^2}{L^2}, \\ x_0 &\equiv \frac{m\, r_{\text{cm}}}{M}. \end{aligned}$$

where $x_0$ is the distance scale of the swing motion.

While the model captures the synchronization and chimera behavior qualitatively, exact quantitative agreement cannot be expected due to inevitable approximations in describing the metronome dynamics. Specifically, the van-der-Pol term describing the metronome escapement is ad-hoc; small scale variations in the center mass motion of the single metronome-swing system are neglected (Eq. 24). Other sources of the discrepancy may be found in the parametrization of the first and second moments of the metronome pendulum mass. Nevertheless, the model captures all physical aspects of our experimental system very well.

## 5 Numerical simulations

The model is a differential algebraic equation (DAE) (Ref. [51]) with $4N+4$ variables. For numerical integration, we have used Mathematica that provides solvers for (implicit) DAEs (including solvers for the initial conditions that need to be consistent with the differential equations to be solved). Mathematica's DAE solver is based on the IDA solver (Refs. [48, 49, 50]).

Rescaling the swing angles by $\tilde{\Phi} = L/x_0\,\Phi$ in the equations is advantageous for numerical integration:

$$\partial_\tau^2 \tilde{\Phi} = \frac{\kappa}{\omega^2}(\tilde{\Psi} - \tilde{\Phi}) - \frac{\Omega^2}{\omega^2}\tilde{\Phi} - \mu_s \partial_\tau \tilde{\Phi} - \sum_{j=1}^{N} \partial_\tau^2 \sin\phi_j, \tag{33}$$

$$\partial_\tau^2 \tilde{\Psi} = \frac{\kappa}{\omega^2}(\tilde{\Phi} - \tilde{\Psi}) - \frac{\Omega^2}{\omega^2}\tilde{\Psi} - \mu_s \partial_\tau \tilde{\Psi} - \sum_{j=1}^{N} \partial_\tau^2 \sin\psi_j, \tag{34}$$

$$\partial_\tau^2 \phi_i = -\sin\phi_i - \mu_m\,\partial_\tau\phi_i\left[\left(\frac{\phi_i}{\theta_0}\right)^2 - 1\right] - \beta\cos\phi_i\,\partial_\tau^2\tilde{\Phi}, \tag{35}$$

$$\partial_\tau^2 \psi_i = -\sin\psi_i - \mu_m\,\partial_\tau\psi_i\left[\left(\frac{\psi_i}{\theta_0}\right)^2 - 1\right] - \beta\cos\psi_i\,\partial_\tau^2\tilde{\Psi}. \tag{36}$$

Here we have introduced the following non-dimensional parameters:

$$\begin{aligned}
\mu_m &\equiv \frac{\nu_m}{I\,\omega}, \\
\mu_s &\equiv \frac{\nu_s}{M\,\omega}, \\
\beta &\equiv \frac{x_0\,\omega^2}{g} = \frac{(m\,r_{\rm cm})^2}{M\,I} = \frac{m}{M}\cdot\frac{m\,r_{cm}^2}{I}, \\
\omega_r^2 &\equiv \frac{\Omega^2}{\omega^2} = \frac{g}{L\,\omega^2} = \frac{I}{m\,L\,r_{\rm cm}}, \\
\chi &\equiv \frac{\kappa}{\omega^2} = \frac{k}{M}\left(\frac{l}{L}\right)^2 \frac{I}{m\,g\,r_{\rm cm}}.
\end{aligned}$$

Parameters $I$ and $r_{\rm cm}$ are parameterized as functions of the nominal frequency $f$ [see Eqns. (7,9,10)], which is one of the two control parameters in our experiment. These parameters may be interpreted as follows. $\beta$ is the ratio of the first and second moments of the metronome and swing masses and determines how much energy is transferred between metronome and swing, thus controlling the the coupling strength between metronomes in a single population; $\chi$ is the spring coupling strength between the populations. The swing energy is dissipated at a rate $\mu_s$. The metronome is characterized by $\mu_m$ and the standard displacement angle $\theta_0$ which tunes how nonlinear the metronome is (note that $\theta_0$ can only be scaled into the metronome and swing angles if $\theta_0 \ll 1$).

Parameters in our experiment are typically:

$$\begin{aligned}
N &= 15 \\
m_s &= 0.915 \text{ kg} \\
m_m &= m_{\rm box} + m_p + m_{\rm bob} = 0.093 \text{ kg} \\
M &= m_s + N \times m_m = 2.31 \text{ kg} \\
m &= m_p + m_{\rm bob} = 0.028 \text{ kg} \\
g &= 9.81 \text{ m. s}^{-2}
\end{aligned}$$

$$
\begin{aligned}
L &= 0.22 \text{ m} \\
L_p &= 0.2 \text{ m} \\
l &= 0.15 \text{ m} \;\; (\, 0.05 \text{ m} \leq l \leq 0.25 \text{ m} \,) \\
f &= 160 \text{ bpm} \;\; (\, 40\,\text{bpm} \leq f \leq 208\,\text{bpm} \,) \\
\omega_n &= 8.38 \text{ rad. s}^{-1} \\
\omega &= 8.61 \text{ rad. s}^{-1} \\
\theta_0 &= 19 \text{ deg} = 0.33 \text{ rad} \\
\Phi^* &= 8.5 \text{ deg} = 0.15 \text{ rad} \\
k &= 68 \text{ N. m}^{-1} \\
\nu_s &\sim 0.1 \text{ kg.s}^{-1} \\
\nu_m &= 1.8 \times 10^{-6} \text{ kg.m}^2\text{.s}^{-1}
\end{aligned}
$$

Note that $\nu_s$ and $\nu_m$ have dissimilar units. The value of $\mu_m$ is based on values obtained from Pantaleone (Ref. [42]). With the above values the non-dimensional parameters are of the following order:

$$
\begin{aligned}
\mu_s &= 0.00016 \\
\mu_m &= 0.011 \\
\beta &= 0.0005 \\
\omega_r^2 &= 0.6 \\
\chi &= 0.092,
\end{aligned}
$$

which are roughly representative of our experiment (see Figs. 2 and 3 in main text).

## Initial conditions

Initial conditions were prepared to be consistent with three types of states: (i) fully synchronized consistent with the IP mode or (ii) the AP mode, or (iii) with chimera states where only one population is synchronized and the other is desynchronized. For the synchronized states (i, ii), we use

$$
\begin{aligned}
\phi_i(0) &= 2\theta_0 \\
\partial_\tau \phi_i(0) &= 0 \\
\psi_i(0) &= \pm 2\theta_0 \\
\partial_\tau \psi_i(0) &= 0, \quad i = 1 \ldots N,
\end{aligned} \tag{37}
$$

where the minus signs apply for the AP mode. For chimera states (iii), the desynchronized population is randomized as follows:

$$
\begin{aligned}
\phi_i(0) &= 2\theta_0 (r_i - 1/2) \\
\phi_i'(0) &= 2\theta_0 (r_i - 1/2), \quad i = 1 \ldots N
\end{aligned} \tag{38}
$$

where $r_i$ is a random number in $[0, 1]$. One may then assign average angles and angular velocities to the synchronized population so that kinetic and potential energy of metronome populations A and B match. For all three types of conditions, the swings are released from their equilibrium positions with zero momentum:

$$
\begin{aligned}
\tilde{\Phi}(0) &= \tilde{\Psi}(0) = 0 \\
\partial_\tau \tilde{\Phi}(0) &= \partial_\tau \tilde{\Psi}(0) = 0.
\end{aligned} \tag{39}
$$

## Integration of model equations and parameter sweeps

Simulations were carried out with identical metronomes until a (quasi-) stationary state was reached ($\tau \sim 12'000$). The stability diagram in the main text (Fig. 4A) was obtained by fixing the nominal metronome frequency $f$ (138, 160, 184 208 bpm) and then gradually increasing the effective spring rate $\kappa$ (using the same parameters as in the experiment and $N = 15$ metronomes per swing). For each parameter step of the sweep simulations were re-initialized with the initial conditions consistent with IP, AP or chimera states as listed above.

The resulting phase diagram does not represent observed states in comprehensive detail, but is a simplified view of a complex spectrum of states. IP and AP states always represent perfectly synchronized states; the region of chimera-like states comprise any states where at least one population is perfectly synchronized. A detailed stability analysis would be needed to uncover further questions including precise stability properties and bifurcation scenarios of these states.

## Further simulations

In order to extend our experiments, we also carried out simulations for situations which are not possible (or are very difficult) to achieve experimentally. We mainly carried out two sets of extended simulations: (i) to investigate the effect of dissipation (in this case, the friction of the swing) on the chimera behavior and (ii) to study the transition between the different regions by using increased number of metronomes to reduce finite size fluctuations.

**The effect of swing friction $\nu_s$.** We sought to investigate the effect of swing friction on the chimera region in simulations. For these simulations, we use parameters as listed in the previous section and vary the swing friction by three orders of magnitude from $\nu_s = 0.031$ kg/s to $\nu_s = 3.1$ kg/s. A series of phase diagrams are plotted in Figure S6 for increasing values of $\nu_s$. While the qualitative behavior remains the same in all cases, it can be seen that with increasing friction, the width of the region with unsynchronized (chimera-like) behavior increases, further demonstrating that the difference between the experimental and numerical phase diagrams in the main text (see Fig. 3) could come due to such effects.

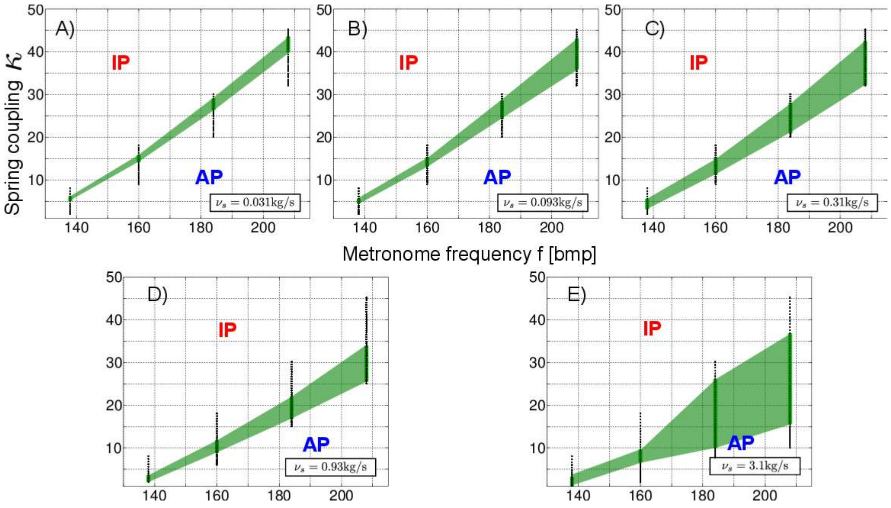


Fig. S 6: Phase diagrams with varying swing friction $\nu_s$. The green shaded region displays the region where one asynchronous population exists. Black dots denote sampled points in parameter space.

**Simulations with $N = 64$ metronomes.** The transition of chimeras between AP and IP regions is investigated with an increased number of metronomes to reduce finite size fluctuations (see Fig. 4 in main text). The modification of the parameters as listed below corroborates that the chimera phenomenon is not specific to a small parameter region.

$$\begin{aligned} f &= 184 \\ \omega_r^2 &= 0.38 \\ \chi &= 0.294 \ldots 0.266 \\ \tilde{\beta} &= 0.00031 \\ \mu_s &= 0.002 \\ \mu_m &= 0.0092 \\ \theta_0 &= 0.66. \end{aligned}$$

# References


[41] Matthew Bennett, Michael Schatz, and Kurt Wiesenfeld. Huygen's clocks. *Proc. R. Soc. London A*, 458(2019):563, 2002.

[42] James Pantaleone. Synchronization of metronomes. *American Journal of Physics*, 70(10):992, 2002.

[43] Steven H. Strogatz. *Nonlinear Dynamics And Chaos.* Perseus Books Publishing, 1994.

[44] Arkady Pikovsky, Michael Rosenblum, and Jürgen Kurths. *Synchronization. A universal comcept in nonlinear sciences.* Cambridge University Press, 2001.

[45] Björn Kralemann, Laura Cimponeriu, Michael Rosenblum, Arkady Pikovsky, and Ralf Mrowka. Phase dynamics of coupled oscillators reconstructed from data. *Physical Review E*, 77(6), June 2008.

[46] V. N. Belykh and E. V. Pankratova. Chaotic dynamics of two Van der Pol-Duffing oscillators with Huygens coupling. *Regular and Chaotic Dynamics*, 15(2-3):274–284, April 2010.

[47] Henning Ulrichs, Andreas Mann, and Ulrich Parlitz. Synchronization and chaotic dynamics of coupled mechanical metronomes. *Chaos (Woodbury, N.Y.)*, 19(4):043120, December 2009.

[48] A. Hindmarsh and A. Taylor. *User Documentation for IDA: A Differential-Algebraic Equation Solver for Sequential and Parallel Computers. Lawrence Livermore National Laboratory.* Technical report, 1999. http://acts.nersc.gov/sundials/documents/237206.pdf

[49] Mathematica:IDA Method for NDSolve. *Wolfram Research.* http://reference.wolfram.com/mathematica/tutorial/NDSolveIDAMethod.html

[50] Mathematica: Numerical Solution of Differential-Algebraic Equations. *Wolfram Research.* http://reference.wolfram.com/mathematica/tutorial/NDSolveIntroductoryTutorialDAEs.html.

[51] Scholarpedia: Differential-algebraic equations http://www.scholarpedia.org/article/Differential-algebraic_equations
